# Supplementary material for: Correcting for the effects of the point spread function in intra-halo light measurements and application to deep Hyper Suprime-Cam data
Source: arXiv:2505.24395 source file (2026-11-06)
Supplement: Supplementary file 1 [file AppendixA.tex]

Due to the method used to construct our dataset of HSC-GAMA mock group observations, we recreate the galaxies in the mocks using the galaxy segmentation maps from the WAVES photometry. In some few cases, these segments are overly extended, as shown in the left panel of Fig.~\ref{G200196}, which corresponds to the mock generated using the configuration of the GAMA group identified by ID G200196. In other few cases, the fragments of bright stars are considered as galaxy segments, and consequently in our mocks, as shown in the left panel of Fig.~\ref{G100224}. In both cases, bright and extended objects can bias our IHL estimations even after applying the PSF correction. Both right panels of Fig.~\ref{G200196} and \ref{G100224} show the flux comparison (upper plot) and the effective radius comparison (lower plot) between the injected and fitted values, where we see how \textsc{ProFit} struggles to find the correct parameters. Fortunately, these are only a few isolated cases in our dataset of mocks and do not significantly affect the median IHL estimations.

\begin{figure*}
\centering  %\qquad
 \includegraphics[width=1\linewidth]{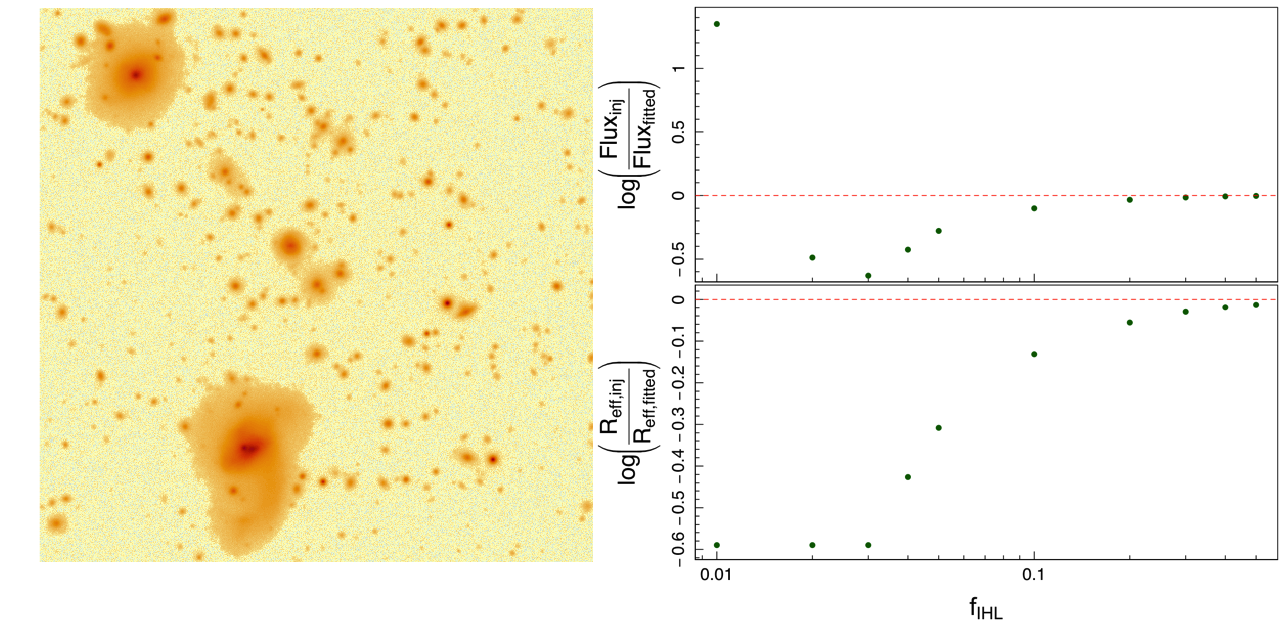}
    \caption{Case study of the mock constructed using the GAMA group configuration from G200196, where extended objects present in the image bias the IHL fitted parameters.}
    \label{G200196}
\end{figure*}

\begin{figure*}
\centering  %\qquad
 \includegraphics[width=1\linewidth]{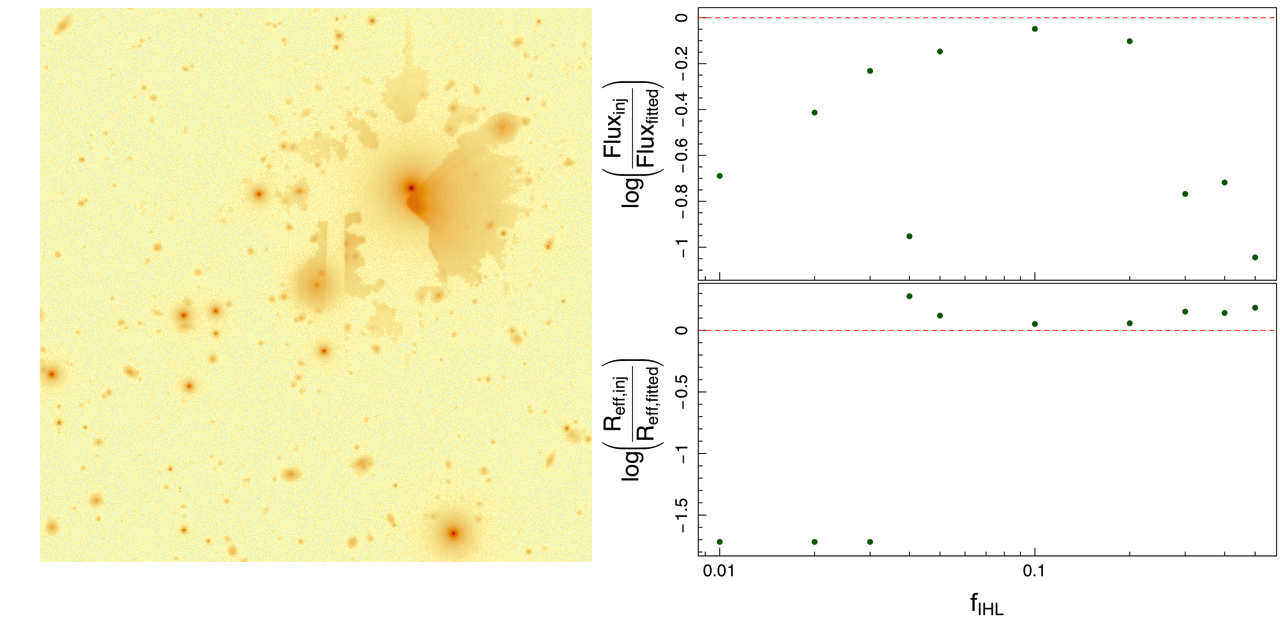}
    \caption{Case study of the mock constructed using the GAMA group configuration from G100224, where fragmented segments of a bright star present in the image bias the IHL fitted parameters.}
    \label{G100224}
\end{figure*}
